# Supplementary material for: Fast Exact Booleans for Iterated CSG using Octree-Embedded BSPs
Source: arXiv:2103.02486 source file (2021-03-03)
Supplement: Supplementary file 1 [file paper-08-appendix.tex]

\section{256 bit arithmetic}

\TODO{multiplication tables for required operations}

\TODO{table for more tradeoffs? like 128bit total logic?}
